# Supplementary material for: Automatically Identifying Parameter Constraints in Complex Web APIs: A Case Study at Adyen
Source: arXiv:2102.00871 source file (2021-02-01)
Supplement: Supplementary file 1 [file appendix.tex]

\subsection{Case Study - Challenge Groups}\label{chapter:challenge_group_tables}
\begin{table}[h]
\caption{High-level reasons for failing to detect constraints for doc analysis.}
\label{table:categorization_table}
\begin{tabularx}{\columnwidth}{|P{1cm}|l|X|}
\bottomrule
\textbf{Code} & \textbf{Short Description}            & \textbf{Description}                                                                        \\ \midrule
A.1  & No info.           			& No information about the constraint in the API reference.            \\ \hline
A.2  & Implicit Info.            	& The constraint was described, but the respective parameters were not referenced directly.       \\ \hline
A.3  & Value not detected. 	& The value the constraint depends on  was not detected.                          \\ \hline
A.4  & Validation           		& Validation requests failed due to unobserved constraints.           \\ \toprule
\end{tabularx}
\end{table}

\begin{table}[h]
\caption{High-level reasons for failing to detect constraints for code analysis.}
\label{table:categorization_table2}

\begin{tabularx}{\columnwidth}{|P{1cm}|l|X|}
\bottomrule
\textbf{Code} & \textbf{Short Description}                 & \textbf{Description}                                                                        \\ \midrule
B.1  & Detection           		& Parameter was accessed, but not detected because it was not in the OpenAPI specification.             \\ \hline
B.2  & Dereferenced           	& Parameter was detected, but dereferenced in variable assignment or object creation.            \\ \hline
B.3  & Variable Stack 			& The value of a variable could not be resolved or be maintained fully statically.                          \\ \hline
B.4  & Preconditions 			& An expression or function imposes a precondition that can not fully be evaluated. E.g boolean cvcRequired = cvcRequired(type)                          \\ \hline
B.5  & Control Structure     	& A control statement such as ‘For, switch, try/catch’ was not handled fully. \\ \hline
B.6  & Data Flow       			& A constraint was missed due to the analysis not being data flow sensitive.       \\ \hline
B.7  & Arithmetic      			& Some constraints with arithmetic syntax are not fully supported. E.g. A + B + … = X   \\ \hline
B.8  & Framework                & Functionality specific to the API framework was used and caused limitation in extracting constraints. \\ \toprule
\end{tabularx}
\end{table}
\vspace{2mm}
\subsection{Documentation Analysis - Word Embeddings}\label{chapter:word_embeddings}
We explored the usage of word embeddings \cite{mikolov2013distributed} as a means to find candidates. Using these vectors, we can obtain a semantic similarity between words, and sentences. The premise is that parameters with semantically similar descriptions are more likely to be related to each other in a constraint.

For every parameter, we calculated its semantic similarity to all other parameters of an endpoint. This allows us to create a list of the most similar parameters for each parameter. If the semantically similar parameters are more likely to be related in constraints, then exploring the most similar parameters would allow us to find constraints without having to exhaust all parameters.

In this process we used SpaCy\footnote{\url{https://spacy.io}} for our word embeddings and similarity measures. We used the $en\_core\_web\_sm$ model, which contains vectors trained on written text such as blogs, news, and comments. For similarity, we used SpaCy's default similarity method for sentences. This method assumes a bag-of-words model for sentences, where the vector of a sentence is the average of the vectors of each word. The similarity between sentences is then determined with the cosine similarity between the two vectors.

In order to test the premise, we used the ground-truth to see the position parameters involved in constraints would have in the list of most similar parameters. For each constraint in the ground truth, we made pairs of related parameters. E.g. for $or(card, bank)$ the pair [card, bank] and for $tenderReference \rightarrow uniqueTerminalId$ the pair [tenderReference, uniqueTerminalId]. Then for every pair we determined the minimum ranking the parameter would have in the other's similarity list between the two parameters. For example, assume that \textit{bank} is on position 8 in \textit{card}'s list and \textit{card} is position 5 on \textit{bank}'s list, then 5 is the rank used for the results shown in Table \ref{table:embedding_results}.

\begin{table*}[t]
\centering

\caption{Table showing the ranking and theoretical number of requests needed when using word embeddings as a similarity measure. The \textit{ranks} column shows the individual ranks of relevant parameters, the \textit{\#Params} the number of parameters for the given endpoint, and \textit{\#Requests} the number of requests needed to validate all candidates.}
\label{table:embedding_results}
\begin{tabular}{|l|P{2.5cm}|l|l|}
\bottomrule
\textbf{Endpoint}        & \textbf{Ranks}               & \textbf{\#Params} & \textbf{\#Requests} \\ \midrule
/payments                & 6, 21, 8, 22                                 & 371                   & 73458                \\ \hline
/authorise               & 51, 21, 3, 8, 324, 1, 6, 20                    & 378                   & 74844                \\ \hline
/capture                 & 31, 1, 18, 8                                   & 192                   & 38016                \\ \hline
/storeDetailAndSubmit... & 1, 1                                           & 51                    & 10098                 \\ \hline
/createAccountHolder     & 3, 2, 67                                        & 103                   & 20394                 \\ \hline
/updateAccountHolder...  & 1                                               & 3                     & 54                  \\ \hline
/createAccount           & 1                                               & 4                     & 108                 \\ \hline
/uploadDocument          & 1                                              & 7                     & 378                 \\ \hline
/getCostEstimate         & 1                                              & 22                    & 4158                 \\ \hline
Total:                   & -                                             & -                     & 221508                \\ \toprule
\end{tabular}
\end{table*}

Looking at the results in Table \ref{table:embedding_results}, we can observe that the rank of relevant parameters is typically within the top 22. This heuristic allows us to filter the search space significantly. Using the formulas provided in section \ref{sec:combinations}, we can calculate the number of requests needed if for every parameter we check the top 22 most similar parameters. For simplicity, we assume every parameter has two values, as such the number of requests is given by $22*P*3^2$, where $P$ is the number of parameters in an endpoint. For every endpoint the number of requests needed to validate all the candidates is given in the \textit{\#Requests} column.

Following these calculations, we would have to make 221508 requests in order to find most constraints that include 2 parameters, which given 5 requests a second would take little over 12 hours. Largely due to the large number of candidates, even for constraints which only include 2 parameters, the approach is rendered impractical.
